# Supplementary material for: TENET: Time-point Encoding Network for Multivariate Time Series Anomaly Detection
Source: arXiv:2610.32337 source file (2026-10-23)
Supplement: Supplementary file 1 [file appendix_title.tex]

\setcounter{equation}{0}
\setcounter{figure}{0}
\setcounter{table}{0}

\makeatletter
\renewcommand{\theequation}{S\arabic{equation}}
\renewcommand{\thefigure}{S\arabic{figure}}
\renewcommand{\thetable}{S\arabic{table}}
